# Supplementary material for: Exploring Explainability in Video Action Recognition
Source: arXiv:2404.09067 source file (2024-04-13)
Supplement: Supplementary file 1 [file X_suppl.tex]

\clearpage
\setcounter{page}{1}
\maketitlesupplementary

% \begin{figure}[ht]
%     \vspace{-2mm}
%     \centering
%  	\includegraphics[width=0.8\linewidth]{figs/GradCAM.png}
%  	\captionsetup{font=small}
%  	\caption{High-level block diagram of Grad-CAM and Grad-CAM with guided backpropagation from~\cite{selvaraju2017grad}. In this work, we restrict ourselves to Grad-CAM, highlighted in the figure.}
%  	\label{fig:gradcam}
% \end{figure}

% \figref{fig:gradcam} shows the high-level block diagram of Grad-CAM, including the guided backpropagation. But for ease of analysis and better visualization, we restrict ourselves to just Grad-CAM. We generate the visualizations using Grad-CAM and superpose the heatmap on the input image to highlight the regions of interest with respect to the prediction of the model as demonstrated in \figref{fig:gradCAM_demo}.

\begin{figure*}[ht]
 \centering 

\begin{minipage}[b]{0.25\linewidth} % Adjust the width to ensure proper spacing
   \centering
   \includegraphics[clip,width=\linewidth]{figs/gradCAM_demo1.png}
   \subcaption{Example input}
 \end{minipage}
 \hspace{0.02\linewidth} % Adjust the horizontal space between the figures
 \begin{minipage}[b]{0.25\linewidth} % Adjust the width to ensure proper spacing
   \centering
   \includegraphics[clip,width=\linewidth]{figs/gradCAM_demo2.png}
   \subcaption{Output of Grad-CAM - \textit{Cat}}
 \end{minipage}
 \hspace{0.02\linewidth} % Adjust the horizontal space between the figures
 \begin{minipage}[b]{0.245\linewidth} % Adjust the width to ensure proper spacing
   \centering
   \includegraphics[clip,width=\linewidth]{figs/gradCAM_demo3.png}
   \subcaption{Output of Grad-CAM - \textit{Dog}}
 \end{minipage}

 \caption{Output of Grad-CAM with respect to different class labels for ResNet-50. In (a), we see the original image that consists of both \textit{cat} and \textit{dog}. In (b), when the Grad-CAM is analyzing the output of ResNet-50 with respect to the class \textit{Cat} and similarly for the class \textit{Dog} in (c).}
 \label{fig:gradCAM_demo}
 \end{figure*}
